# Supplementary material for: Probabilistic Neural-symbolic Models for Interpretable Visual Question Answering
Source: arXiv:1902.07864 source file (2019-06-27)
Supplement: Supplementary file 1 [file appendix_main.tex]

%%%%%%%% PROBABILISTIC NEURAL SYMBOLIC VQA APPENDIX %%%%%%%%%%%%%%%%%

\documentclass{article}

% Recommended, but optional, packages for figures and better typesetting:
\usepackage{microtype}
\usepackage{graphicx}
\usepackage{subfigure}
\usepackage{booktabs} % for professional tables

% hyperref makes hyperlinks in the resulting PDF.
% If your build breaks (sometimes temporarily if a hyperlink spans a page)
% please comment out the following usepackage line and replace
% \usepackage{icml2019} with \usepackage[nohyperref]{icml2019} above.
\usepackage{hyperref}

% Attempt to make hyperref and algorithmic work together better:

\usepackage{hyperref}
\usepackage{url}
\usepackage{amsmath}
\usepackage{relsize}

% Custom defined packages in addition to default ones.
%\usepackage{algorithm}
\usepackage{amsfonts}
\usepackage{multirow}
\usepackage{array}
\usepackage{color}
\usepackage[colorinlistoftodos,prependcaption,textsize=tiny]{todonotes}
\usepackage{amsthm}

\usepackage{xcolor} % Colored text.
\usepackage{xspace}
\usepackage{comment}
\usepackage[noabbrev,capitalize]{cleveref}

% list management
\usepackage{enumitem}
\usepackage[olditem,oldenum]{paralist}

%\algdef{SE}[SUBALG]{Indent}{EndIndent}{}{\algorithmicend\ }%
%\algtext*{Indent}
%\algtext*{EndIndent}

% Use the following line for the initial blind version submitted for review:
%\usepackage{icml2019}

% If accepted, instead use the following line for the camera-ready submission:
\usepackage[accepted]{icml2019}

% Custom macros for typesetting.
\input{../macros.tex}

% packed itemize

% A new theorem for the result discussed in the paper.

% The \icmltitle you define below is probably too long as a header.
% Therefore, a short form for the running title is supplied here:
\icmltitlerunning{Appendix}

\marginparsep=11.0pt
\marginparwidth=65.0pt

\begin{document}

\twocolumn[
\icmltitle{Appendix: Probabilistic Neural-symbolic models for \\
Interpretable Visual Question Answering}

% It is OKAY to include author information, even for blind
% submissions: the style file will automatically remove it for you
% unless you've provided the [accepted] option to the icml2019
% package.

% List of affiliations: The first argument should be a (short)
% identifier you will use later to specify author affiliations
% Academic affiliations should list Department, University, City, Region, Country
% Industry affiliations should list Company, City, Region, Country

% You can specify symbols, otherwise they are numbered in order.
% Ideally, you should not use this facility. Affiliations will be numbered
% in order of appearance and this is the preferred way.
\icmlsetsymbol{equal}{*}

% You may provide any keywords that you
% find helpful for describing your paper; these are used to populate
% the "keywords" metadata in the PDF but will not be shown in the document
\icmlkeywords{Machine Learning, ICML}

\vskip 0.3in
]

% this must go after the closing bracket ] following \twocolumn[ ...

% This command actually creates the footnote in the first column
% listing the affiliations and the copyright notice.
% The command takes one argument, which is text to display at the start of the footnote.
% The \icmlEqualContribution command is standard text for equal contribution.
% Remove it (just {}) if you do not need this facility.

%\printAffiliationsAndNotice{}  % leave blank if no need to mention equal contribution
%\printAffiliationsAndNotice{\icmlEqualContribution} % otherwise use the standard text.

% In the unusual situation where you want a paper to appear in the
% references without citing it in the main text, use \nocite
%\nocite{langley00}
	
\input{appendix.tex}

\bibliography{../bib.bib}
\bibliographystyle{icml2019}

\end{document}
